# Supplementary material for: Multi-Objective Quality-Diversity for Crystal Structure Prediction
Source: arXiv:2403.17164 source file (2024-06-21)
Supplement: Supplementary file 1 [file crowding_ablations.tex]

\section{Addition and Selection Ablations}\label{section:crowding_ablations}
