# Supplementary material for: Multi-Objective Quality-Diversity for Crystal Structure Prediction
Source: arXiv:2403.17164 source file (2024-06-21)
Supplement: Supplementary file 2 [file relaxation_appendix.tex]

\section{Relaxation Ablations}\label{section:relaxation_ablations}
