# Supplementary material for: Multi-Objective Quality-Diversity for Crystal Structure Prediction
Source: arXiv:2403.17164 source file (2024-06-21)
Supplement: Supplementary file 3 [file thresholding_ablations.tex]

\section{Thresholding Ablations}\label{section:thresholding_ablations}

\begin{table}[ht]
\centering
  \caption{Median number of reference structure matches}
  \scalebox{0.9}{\begin{tabular}{c|c|c}
    \toprule
    & \makecell{\textbf{With Threshold}}
    & \makecell{\textbf{Without Threshold}} \\

    \midrule

    $C$
    &
    & \\
    
    \midrule

    $Si$
    &
    & \\

    \midrule
    
    $SiC$
    &
    & \\
    
    \midrule
    
    $Si$
    &
    & \\

    \midrule
    $TiO2$
    &
    & \\    
    
    \bottomrule
    
\end{tabular}\label{tab:structure_matcher_results}}

\end{table}

\begin{itemize}
    \item Structure matching to reference structures (archive view and reference view)
    \item Structures grouped by similarity 
\end{itemize}
